# Supplementary material for: Large-size multivariate scale-free texture generation from small-size learning sets with self-attention Wasserstein-GAN
Source: arXiv:2610.29535 source file (2026-10-21)
Supplement: Supplementary file 1 [file appendix.tex]

\appendix

\addcontentsline{toc}{chapter}{APPENDICES}
\section{Appendix}
\section{Results and Discussion}
10 W-GAN and 10 SA-GAN were trained from scratch and the generated images were analysed taking textures of size $2\times128\times 128 $, $2\times512\times 512 $, $2\times1024\times 1024 $.
\input{tables/W-SA-Stat}

In order to see how close we are to the theoretical values we look at:
\input{tables/TableInput}
Or we can look at the distance to the approx values:
\begin{figure}[h]
  \centering
  \includegraphics[trim={2cm 7cm 2cm 7cm}, clip, width=0.22\textwidth]{images/DistanceSlopes/Distance128c1.pdf}%
  \hfill % pushes them to the sides with flexible space
  \includegraphics[trim={2cm 7cm 2cm 7cm}, clip, width=0.22\textwidth]{images/DistanceSlopes/Distance128c2.pdf}
  \includegraphics[trim={2cm 7cm 2cm 7cm}, clip, width=0.22\textwidth]{images/DistanceSlopes/Distance1024c1.pdf}%
  \hfill % pushes them to the sides with flexible space
  \includegraphics[trim={2cm 7.2cm 1.6cm 7cm}, clip, width=0.22\textwidth]{images/DistanceSlopes/Distance1024c2.pdf}
  \caption{Left: Evolution of $||c_1-c_1Theo||$ per epoch, 
  Right: Evolution of $||c_2-c_2Theo||$ per epoch.}
  \label{fig:pdf-example}
\end{figure}

We average 10 realizations and show how the c1 and c2 slopes are being finded:
\input{figures/c1}
\input{figures/c2}
\input{figures/rho_rhomf}
% \begin{figure}[h]
%   \centering
%   \includegraphics[trim={3.5cm 9cm 5cm 9cm}, clip, width=0.22\textwidth]{images/Stats/c1_1.pdf}%
%   \hfill % pushes them to the sides with flexible space
%   \includegraphics[trim={3.5cm 9cm 5cm 9cm}, clip, width=0.22\textwidth]{images/Stats/c1_2.pdf}
%   \includegraphics[trim={3.5cm 8.5cm 5cm 9cm}, clip, width=0.22\textwidth]{images/Stats/c2_1.pdf}%
%   \hfill % pushes them to the sides with flexible space
%   \includegraphics[trim={3.5cm 8.5cm 5cm 9cm}, clip, width=0.22\textwidth]{images/Stats/c2_2.pdf}
%   \includegraphics[trim={3.5cm 8.5cm 5cm 9cm}, clip, width=0.22\textwidth]{images/Stats/rho.pdf}
%   \includegraphics[trim={3.5cm 8.5cm 5cm 9cm}, clip, width=0.22\textwidth]{images/Stats/rho_MF.pdf}
%   \caption{Average}
%   \label{fig:pdf-example}
% \end{figure}
% \begin{figure}
%     \centering
%     \includegraphics[width =\linewidth]{images/DistanceSlopes/128mean_std_compare_aprox.jpg}
%     \includegraphics[width =\linewidth]{images/DistanceSlopes/1024mean_std_compare_aprox.jpg}
%     \caption{Caption}
%     \label{fig:my_label}
% \end{figure}


\begin{figure}[htbp]
    \centering
    \adjustbox{trim=0pt 0pt {0.5\linewidth} 0pt, clip}{\includegraphics[width=\linewidth]{images/generated/1024/BestW1024.png}}%
    \adjustbox{trim={0.125\linewidth} 0pt 0pt 0pt, clip}{\includegraphics[width=0.25\linewidth]{images/generated/128/BestW128.png}}
    \caption{Best WGAN 128 $H, \lambda^2 =0.792,  0.018$, 1024  $H, \lambda^2 =0.808,  0.015$ }
\end{figure}
\begin{figure}[htbp]
    \centering
    \adjustbox{trim=0pt 0pt {0.5\linewidth} 0pt, clip}{\includegraphics[width=\linewidth]{images/generated/1024/WorstW1024.png}}%
    \adjustbox{trim={0.125\linewidth} 0pt 0pt 0pt, clip}{\includegraphics[width=0.25\linewidth]{images/generated/128/WorstW128.png}}
    \caption{Worst WGAN generated images}
\end{figure}
\begin{figure}
    \centering
    \includegraphics[width=\linewidth]{images/10TrainingCombined/AllRho.png}
    \caption{AllCombined}
\end{figure}
\begin{figure}
    \centering
    \includegraphics[width=\linewidth]{images/10TrainingCombined/AllNoRho.png}
    \caption{AllCombinedNoRho}
\end{figure}
